# Supplementary material for: Gravitational wave luminosity distance-weighted anisotropies
Source: arXiv:2404.12351 source file (2024-10-21)
Supplement: Supplementary file 1 [file Appendix_Numerical_Implementation.tex]

\label{Numerical Implementation}

In this work, we calculate the angular power spectrum of the GR corrections on $\DL$, defined Eqs.~\eqref{total formula pois},~\eqref{Cl general}, by using \texttt{Multi\_class}~\cite{Bellomo:2020pnw,Bernal:2020pwq}, an extension of CLASSgal~\cite{DiDio:2013bqa}, which gives the possibility of computing the angular power spectrum of the cross-correlation between different tracers. According to Eq.~\eqref{DL background}, the GR corrections on the luminosity distance can be decomposed in a term proportional to the corrections on the luminosity distances on the single sources plus the GR corrections on the number of events,
\begin{align}
    C_{\ell}(z_i,z_j)&=4\pi\int \frac{\ud k}{k} P(k) \left(\Delta\ln\DL\right)_{\ell }(z_i) \left(\Delta\ln\DL\right)_{\ell }^{*}(z_j)\nonumber\\
    &=4\pi\int \frac{\ud k}{k} P(k) \left[\Delta_{\ell}^{\D_L}(z_i)+\Delta_{\ell}(z_i)\right]\left[\Delta_{\ell}^{\D_L}(z_j)+\Delta_{\ell}(z_j)\right]^* \, .
    \label{formula Cl sum}
\end{align}
The terms in the round parenthesis are multiplied by the window functions defined in Eq.~\eqref{def:window_functions_V_DL}, which depends on the bin and type of GR correction considered, i.e., corrections on the luminosity distance or on the number count. We modify \texttt{Multi\_CLASS} by introducing a new output, \texttt{LuminosityDistanceCl}, which takes as input the center of the bin and its width $\D_L^{\rm bin}$ and $\sigma^{\rm bin}_{\D_L}$, as in the standard version of \texttt{CLASSgal}, allowing the user to bin also in luminosity distance space and not just in redshift space. The output \texttt{LuminosityDistanceCl} creates two ‘‘tracers'', with the same \texttt{selection\_window} and \texttt{selection\_dNdz}, but with different selection functions computed in the transfer module. The source functions associated to the two tracers are identical, but the source function associated to $\Delta^{\D_L}_\ell$ uses $s=$, while the one related to $\Delta_{\rm GW}$ uses the value computed in Eq.~\eqref{}. It is easy to check indeed that the source function for the luminosity distance, Eq.~\eqref{}, is equivalent to the source function for the number of events, Eq.~\eqref{}, when $s=...$. \LVDA{Inserisci il valore e l'equazione dove definiamo il magnification bias.}
